# Supplementary material for: Neural Video Compression with Diverse Contexts
Source: arXiv:2302.14402 source file (2023-03-14)

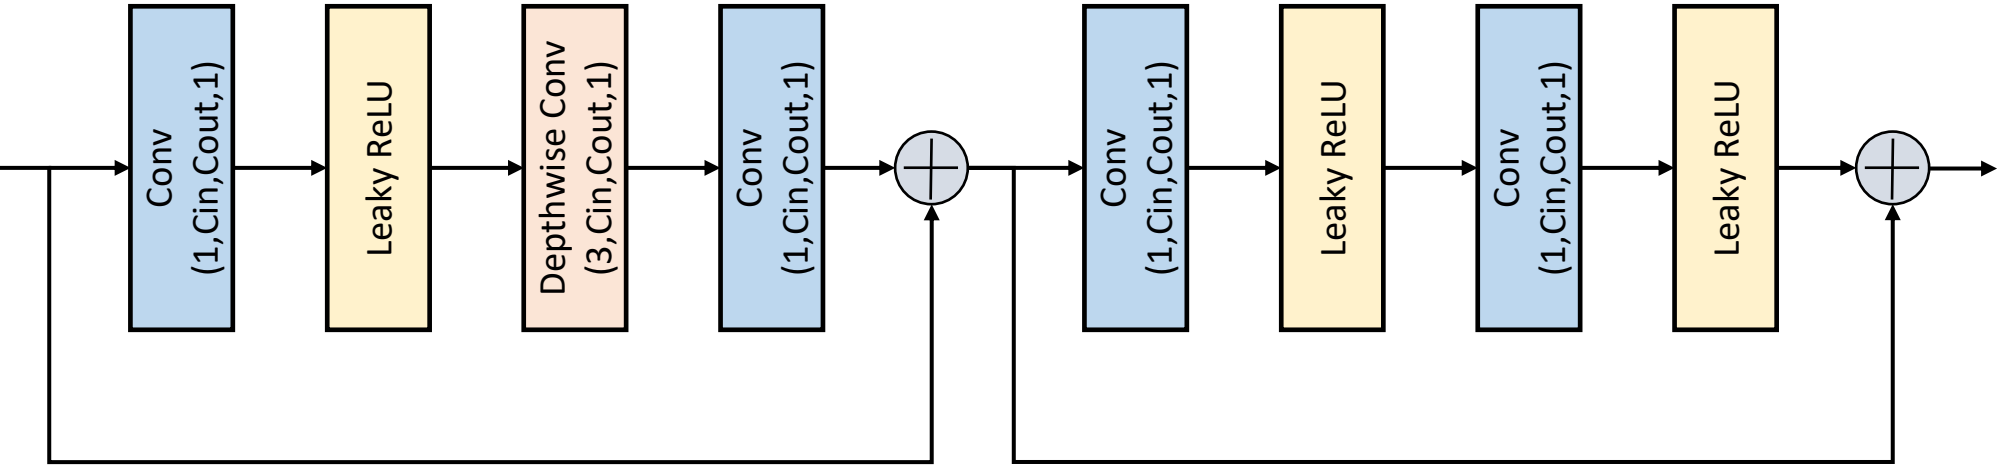

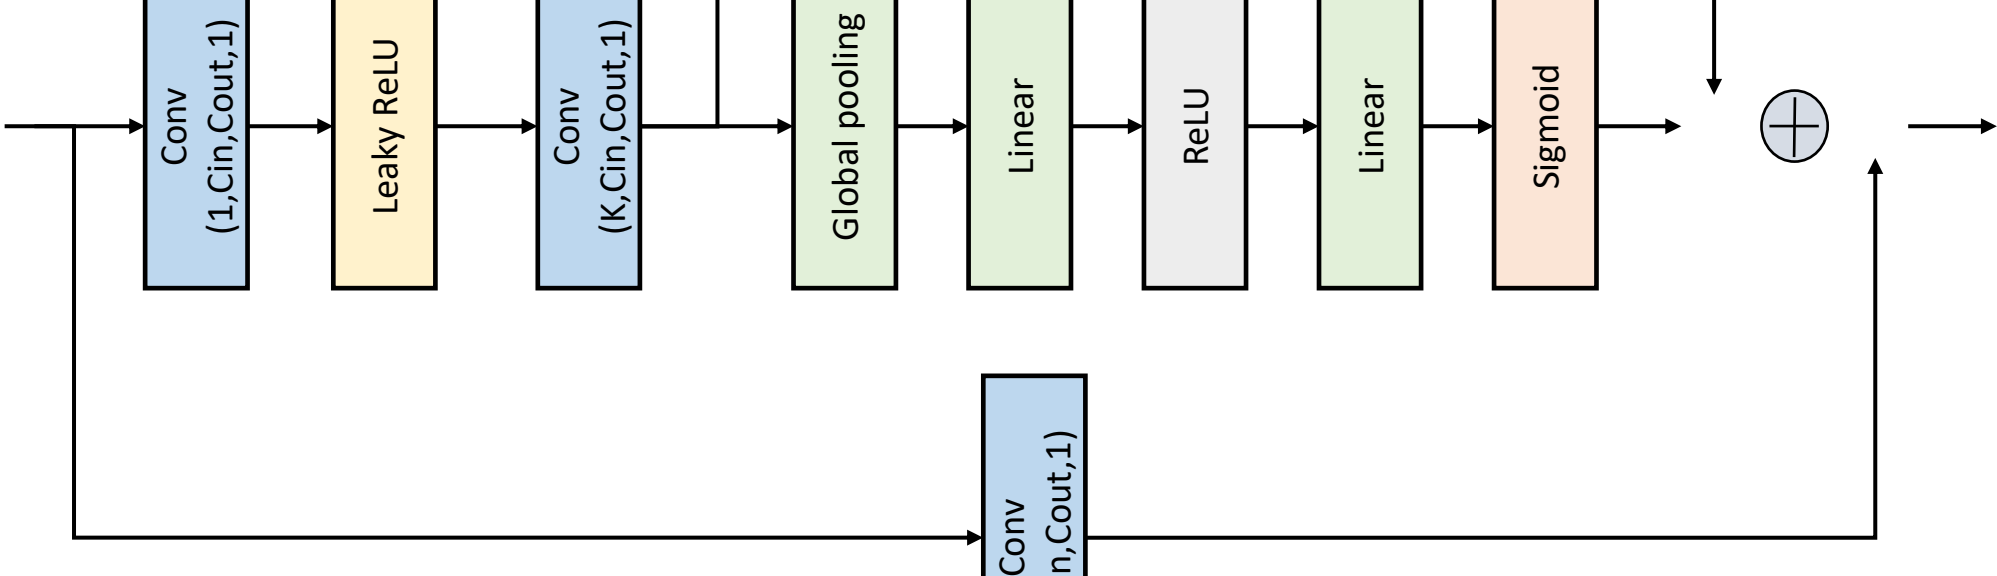

Supplement: Supplementary file 1 [file supp_depthConvBlock.pdf]
