# Supplementary material for: Neural Video Compression with Diverse Contexts
Source: arXiv:2302.14402 source file (2023-03-14)

*decoded  
hyper prior*       $\hat{y}_{t-1}$       *temporal  
context prior*

DepthConvBlock

DepthConvBlock

DepthConvBlock

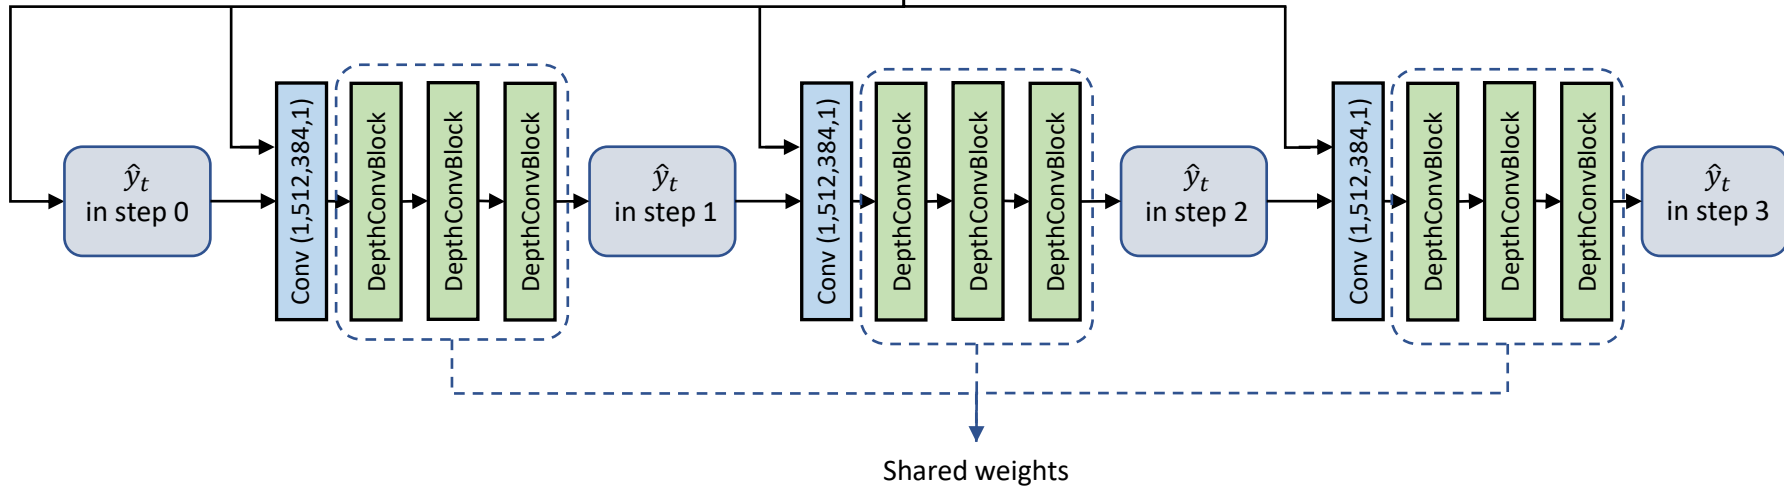

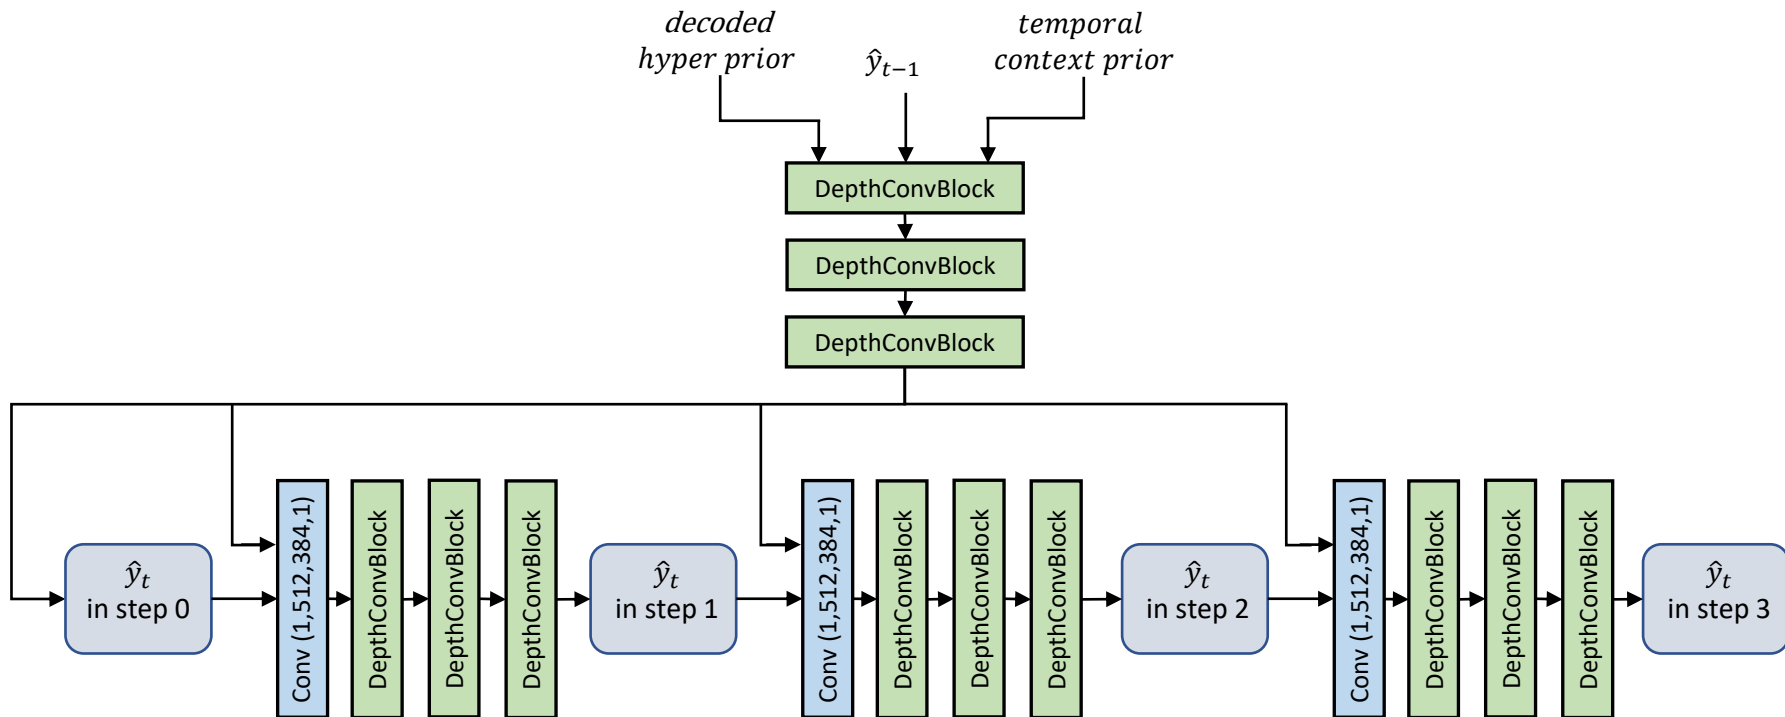

Supplement: Supplementary file 2 [file supp_quadtree_partition.pdf]
